# Supplementary material for: Quantum dynamics simulation of exciton-polariton transport
Source: arXiv:2410.23739 source file (2024-10-31)
Supplement: Supplementary file 1 [file si.pdf]

# Supplementary Information for: Quantum dynamics simulation of exciton-polariton transport

Niclas Krupp,*,† Gerrit Groenhof,‡ and Oriol Vendrell*,†

†*Theoretische Chemie, Physikalisch-Chemisches Institut, Universität Heidelberg, INF 229, 69120 Heidelberg, Germany*

‡*Nanoscience Center and Department of Chemistry, University of Jyväskylä, P.O. Box 35, Jyväskylä 40014, Finland*

E-mail: niclas.krupp@pci.uni-heidelberg.de; oriol.vendrell@uni-heidelberg.de

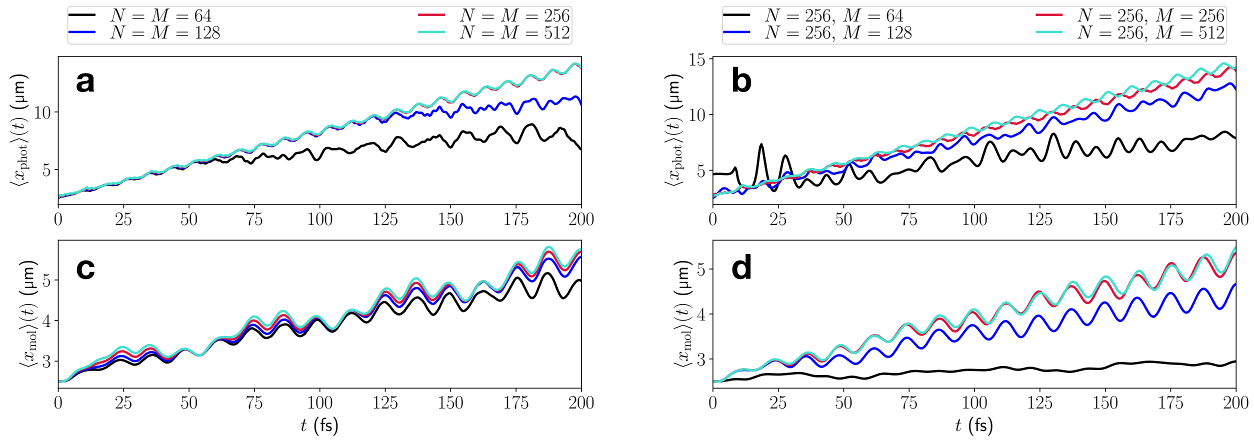


Figure S1: Convergence study. Mean positions of photonic (a,c) and molecular subsystems (b,d) for various numbers of cavity modes ($M$) and molecules ($M$) while keeping the intermolecular distance $\Delta x$ fixed. The cavity coupling strengths $g_j(k_x)$ are scaled by $1/\sqrt{N}$ to keep a constant Rabi splitting of $\hbar\Omega_R = 328\,\mathrm{meV}$.

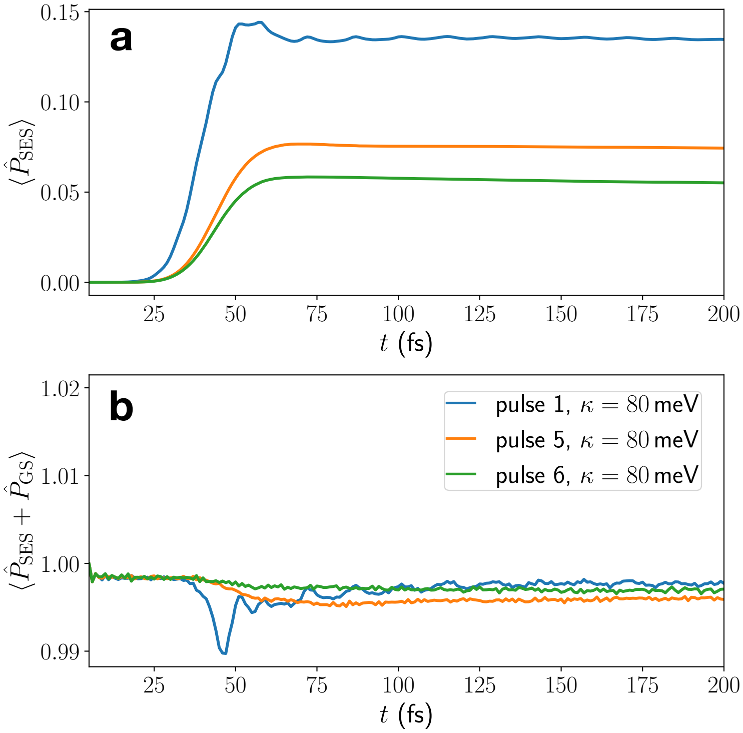


Figure S2: (a) Single-excitation subspace (SES) population and (b) ground-state + SES population after laser excitation for three representative pulses. The SES population stays almost constant after the pulse is over, indicating that the dynamics predominantly occurs within the SES. Leakage to higher-excitation subspaces either due to a breakdown of the rotating wave approximation or high laser intensities is very small, the majority of population resides in the ground-state or SES.

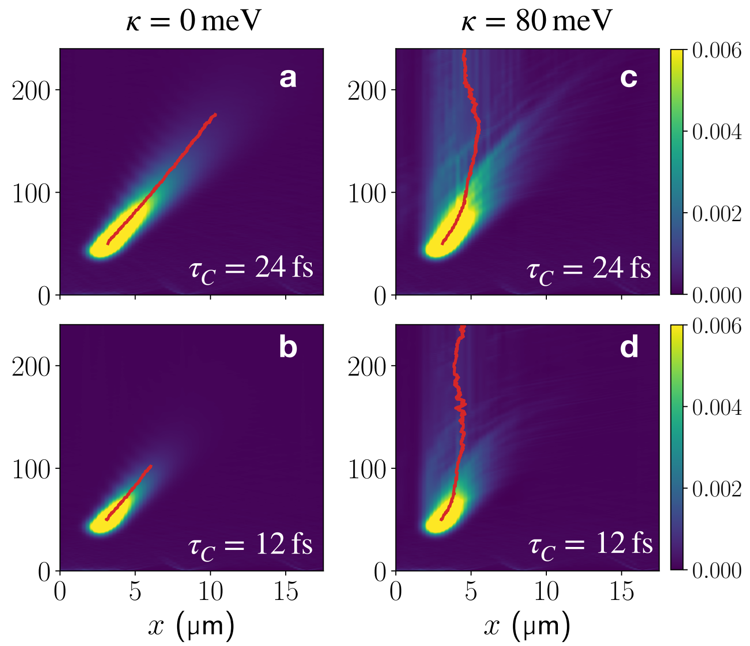


Figure S3: Polariton wavepacket contraction in lossy cavities. Excitation with broad-band laser pulse ($F_t = 10\,\mathrm{fs}$, $k_x^{(0)} = k_x^{\mathrm{res}}$, $\omega_L = 4.351\,\mathrm{eV}$) targeting UP at resonant wavevector. Without (a,b) and with (c,d) vibronic coupling for two cavity mode lifetimes $\tau_C$.
